# Supplementary material for: Closing the superconducting gap in small Pb-nanoislands with high magnetic fields
Source: arXiv:1702.03686 source file (2017-02-13)
Supplement: Supplementary file 1 [file Supporting_Information.pdf]

**Supporting Information**

*dI/dV* FITTING METHOD:

To fit the *dI/dV* spectra the following expression based on the formula of Dynes[1] was used:

$$dI/dV = A \int \frac{\partial f(\epsilon - eV,\, T)}{\partial V}\, n_S(\epsilon)\, \mathrm{d}\epsilon \qquad (S1)$$

$$\text{with:} \quad n_S(\epsilon) = \begin{cases} Re \dfrac{|\epsilon - i\Gamma|}{\sqrt[2]{(\epsilon - i\Gamma)^2 - \Delta^2}} & , \quad \Delta > 0 \\ 1 & , \quad \Delta = 0 \end{cases}$$

The voltage region above $V = \pm$ 1.2 mV is strongly influenced by different effects which we attribute to the observed disorder and phonon excitations in the islands. Since the Dynes formula do not account for those effects for each *dI/dV* fit in the main text, and in Figure S1 and Figure°S2, only the voltage region of $V = \pm$ 1.2 mV around zero bias was used for the fitting. The fitting parameters were the amplitude $A$, the broadening $\Gamma$ and the superconducting gap $\Delta$. $f(\epsilon, T)$ is the Fermi-Dirac distribution. As explained in Fig S1, the temperature $T$ was set to 0.6 K.

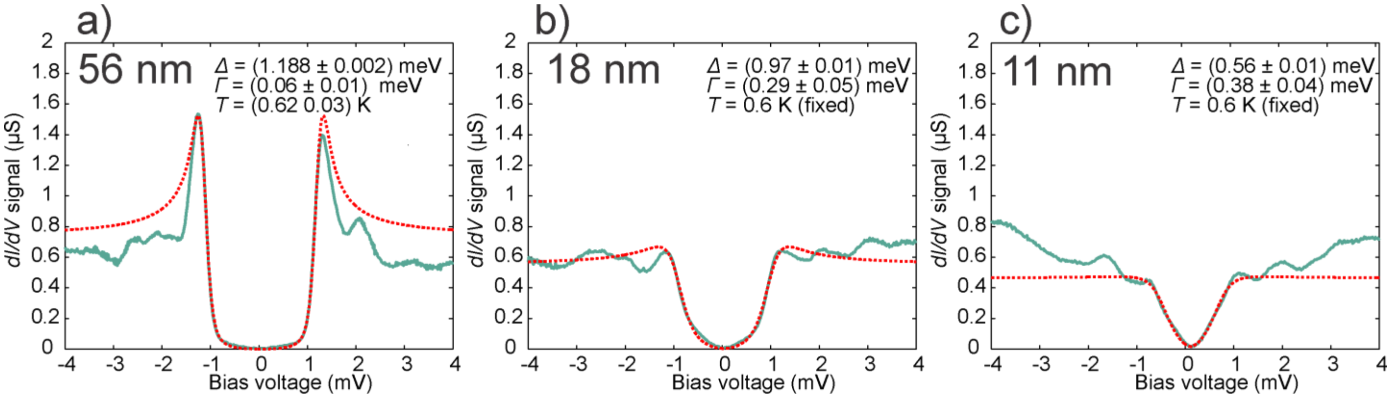


**Figure S1.** Differential conductance spectra (*dI/dV*) of three islands with different diameters $d$ as a function of bias voltage in absence of a magnetic field. All three islands show a

superconducting gap which decreases for smaller islands. **(a)** For the largest island there are pronounced coherence peaks which are suppressed for smaller islands **(b-c)**. (red dotted lines) Each *dI/dV* spectra were fitted based on the Dynes formula, equation S1. For the large island, (a), the temperature *T* was also a fit parameter. The best fit was achieved with T = (0.62 ±0.03) K which matches well to the base temperature of our experiment of 0.6 K. For this reason the temperature parameter *T* was fixed for all other spectra to 0.6 K.

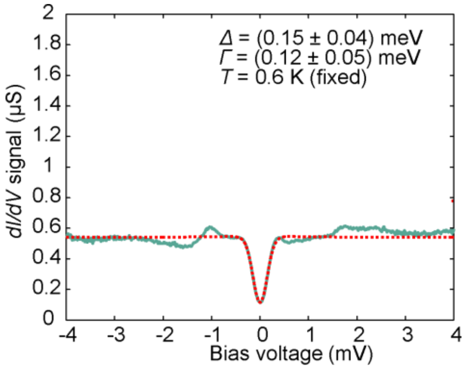


**Figure S2.** *dI/dV* spectra on the Pb wetting layer as the function of bias voltage in absence of a magnetic field. The red dotted line indicates the fit based on the Dynes formula, equation S1.

ANDERSON CRITERION:

Based on the Anderson Criterion one would expect that superconductivity in superconducting particles vanishes if the mean level spacing $\delta$ of the electronic states at the Fermi energy becomes larger as the bulk superconducting gap. The mean level spacing can be approximated by the following formula[2]:

$$\delta = \frac{2\,\pi^2\,\hbar^2}{m_e k_F V} = \frac{95.8}{V[\mathrm{nm}^3]}\,\mathrm{meV} \qquad (S2)$$

With $m_e$ the mass of an electron, $k_F$ the Fermi wave vector (for Pb: $k_F = 1.57\times 10^{10}\,\frac{1}{\mathrm{m}}$ [3]), $V$ the volume. The volume is given by: $V = 7h_0 A = 7h_0\ {\pi d^2}/{4}$, with $h_0$ as the height of one atomic layer (ML) of Pb given by $d_{ML}$ = 0.285 nm[4,5], $A$ the area of the island and $d$ the diameter. Based this calculation, for an island with a 6.7 nm diameter, the mean level spacing is equal of the bulk superconducting gap 1.365 meV[3]. In Table S1 for different islands sizes the approximated mean level spacing is shown.

| Diameter $d$ | Area $A$ | Volume $V$ | Mean Level spacing $\delta$ |
|---|---|---|---|
| 50 nm | 1964 nm$^2$ | 3918 nm$^3$ | 0.02 meV |
| 10 nm | 79 nm$^2$ | 158 nm$^3$ | 0.61 mev |
| 5 nm | 20 nm$^2$ | 40 nm$^3$ | 2.4 meV |
| 6 nm | 28 nm$^2$ | 56 nm$^3$ | 1.70 meV |
| 6.7 nm | 35 nm$^2$ | 70 nm$^3$ | 1.365 meV |

**Table S1**. Approximated mean level spacing $\delta$ for different island sizes

VERIFICATION OF THE $V_e$ METHOD:

We simulated the *dI/dV* spectra as increasing magnetic field $B$, to verify that the $V_e$ method used to extract the critical field in the main text is reasonable. For the simulation we assumed, that:

- The $dI/dV$ is based on the Dynes-formula, equation S1,

- The superconducting gap as function of the $B$-field is given by $\Delta(B) = \Delta_0\sqrt{1-\left(\frac{B}{B_c}\right)^2}$

- The broadening factor $\Gamma$ is constant with changing of the magnetic field.

The simulated $dI/dV$ measurement is shown in Figure S3. A theoretical voltage width $2V_e$, at which the conductance lies below $1/e$ of the average background conductance, $\sigma_b$, was calculated based on the simulated $dI/dV$ curves.

For the parameters used in Figure S4, $\Delta(B)/V_e(B)$ is approximately constant for all magnetic fields close to the critical field, Figure S3c. Only in the immediate vicinity of the superconducting transition (approx. 50mT before the critical field is reached), does the factor $\Delta(B)/V_e(B)$ start to diverge. The fact that it is constant over a large magnetic field window allows the determination of the critical field by $V_e(B)$.

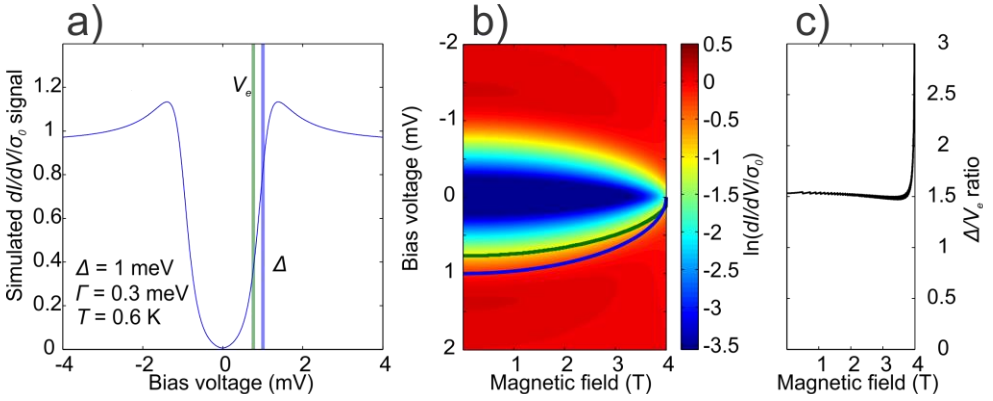


**Figure S3.** The simulated $dI/dV$ spectra. In the simulation the critical field was set to 4 T. **(a) N**ormalized $dI/dV$ spectra at zero magnetic field, the position of the gap $\Delta$ (green vertical line) and of the width $V_e$ (blue vertical line) are marked.**(b)** The simulated superconducting gap $\Delta$ as well as the width $V_e$ closing as function of the magnetic field. The blue and the green lines

indicate the position of the *Δ(B)* and of the width $V_e(B)$ respectively. **(c)** The ratio of $\Delta(B)/V_e(B)$ is approximately constant and only starts to deviate directly when B is close to the critical field (c).

CURRENT DEPENDENCE OF *dI/dV* SPECTRA

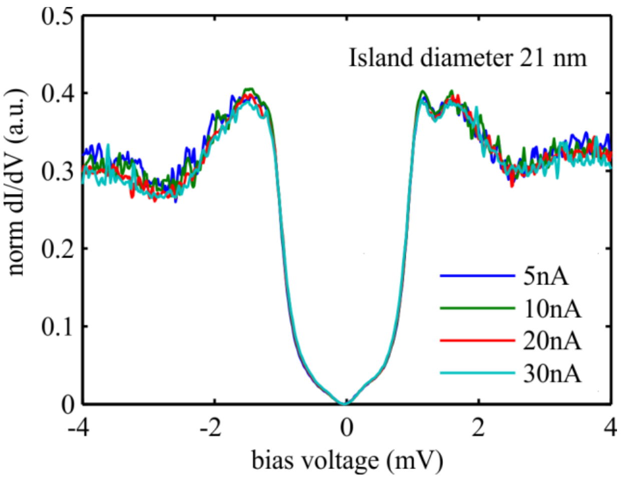


**Figure S4.** Series of current setpoint dependent *dI/dV* spectra performed on a 21 nm diameter island (voltage setpoint +4 mV). The normalized and shifted spectra are completely indistinguishable excluding any additional broadening.

COMPARISON WITH THE ZERO-BIAS-CONDUCTANCE METHOD TO EXTRACT THE CRITICAL FIELD

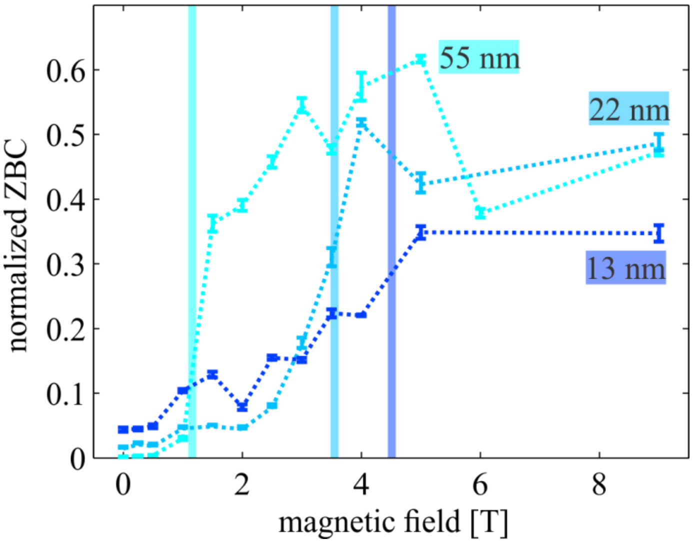


**Figure S5.** In the previous studies the zero bias conductances (ZBC) normalized to the background conductance as function of the applied magnetic field was used to extract the critical magnetic field. To compare the findings of the method used in the main text we extracted the normalized ZBC as function of magnetic field for three different islands. The vertical lines indicate the critical fields based on the $V_e$ width analysis used in the main text. The ZBC saturates around 0.4 of the background conductance when superconductivity breaks down in the corresponding island. The critical fields which one would extract with the help of the ZBC are very close to the values extracted from the $V_e$ width analysis.

RESIDUAL ORDER OF WETTING LAYER

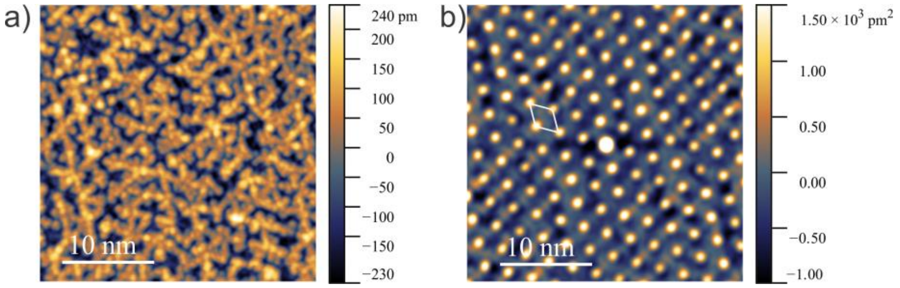


**Figure S6** Residual order of the wetting layer. a) 30nmx30nm topography of the wetting layer. The wetting layer exhibits a residual order which matches to the 7x7 reconstruction of the Si substrate. That the residual order is long range is shown in the autocorrelation b). In the autocorrelation image the unit cell is marked.

**REFERENCES**


(1) Dynes, R. C.; Narayanamurti, V.; Garno, J. P. *Phys. Rev. Lett.* **1978**, *41*, 1509–1512.

(2) Ralph, D. C.; Black, C. T.; Tinkham, M. *Phys. Rev. Lett.* **1995**, *74*, 3241–3244.

(3) Kittel, C. *Introduction to solid state physics*, 7th ed.; John Wiley & Sons, Inc: New York, Chichester, Brisbane, Toronto,Singapore, 1996.

(4) Budde, K.; Abram, E.; Yeh, V.; Tringides, M. C. *Phys. Rev. B* **2000**, *61*, R10602–R10605.

(5) Hupalo, M.; Kremmer, S.; Yeh, V.; Berbil-Bautista, L.; Abram, E.; Tringides, M. *Surface Science* **2001**, *493*, 526 – 538.
